# Supplementary material for: Selected configuration interaction dressed by perturbation
Source: arXiv:1806.04970 source file (2018-07-17)
Supplement: Supplementary file 1 [file ShiftedBk-SI.pdf]

# Supplementary material for “Selected configuration interaction dressed by perturbation”

Yann Garniron,[1] Anthony Scemama,[1] Emmanuel Giner,[2] Michel Caffarel,[1] and Pierre-François Loos[1, a)]

[1)] *Laboratoire de Chimie et Physique Quantiques, Université de Toulouse, CNRS, UPS, France*

[2)] *Laboratoire de Chimie Théorique, Université Pierre et Marie Curie, Sorbonne Université, CNRS, Paris, France*

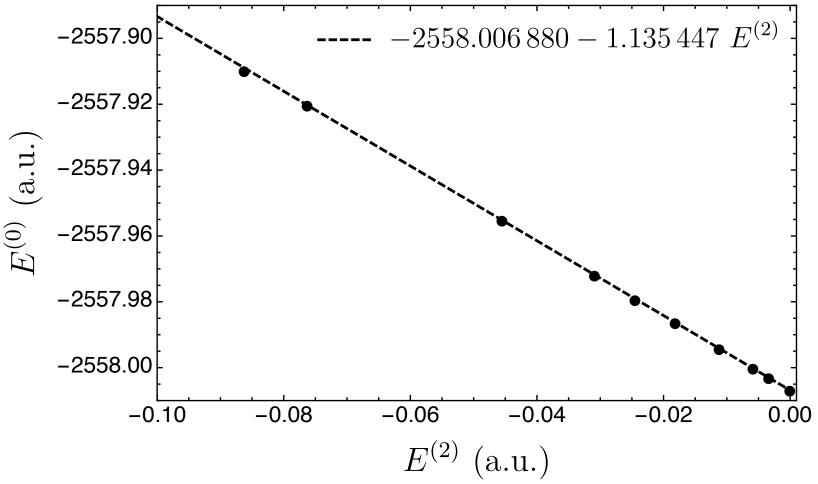


FIG. 1. Extrapolation of the sCI energies to the FCI limit (i.e. $E^{(2)} = 0$) for the ground state of the $CuCl_2$ molecule obtained with the 6-31G basis set. The last two points (corresponding to the the two largest wave functions, that is, having the smallest $E^{(2)}$ values) are taken into account in the linear extrapolation.

TABLE I. Total energies (in hartree) of cyanines for various methods. The error bar corresponding to one standard deviation is reported in parenthesis.

| Method | Ground state | | Excited state | |
|---|---|---|---|---|
| | CN3 | CN5 | CN3 | CN5 |
| CAS($\pi$)[a] | −149.535 876 | −226.477 375 | −149.255 678 | −226.283 870 |
| CAS($\pi$)+PT2 | −150.050 696(0) | −227.231 239(3) | −149.777 783(0) | −227.046 760(4) |
| CAS($\pi$)+sBk$_0$ | −150.052 063(0) | −227.234 134(2) | −149.780 238(0) | −227.051 134(3) |
| CAS($\pi$)+sBk | −150.056 70 | −227.241 99 | −149.793 39 | −227.066 59 |
| exFCI[b] | −150.019 253 | −227.219 823 | −149.755 922 | −227.040 256 |

[a] CAS-CI/aug-cc-pVDZ calculations: CAS(4,32) and CAS(6,50) for CN3 and CN5, respectively.
[b] Extrapolated CIPSI/aug-cc-pVDZ calculations.

[a)]Corresponding author: loos@irsamc.ups-tlse.fr

TABLE II. Zeroth-order energy $E^{(0)}$ and second-order energy $E^{(2)}$ (both in hartree) of the ground and first excited states of CN3 and CN5 as a function of the number of determinants $N_{\text{det}}$ in the sCI expansion. The excitation energies (in eV) are also reported. The error bar corresponding to one standard deviation is reported in parenthesis.

| Molecule | $N_{\text{det}}$ | Ground state | | Excited state | | Excitation energy (eV) |
|---|---|---|---|---|---|---|
| | | $E^{(0)}$ | $E^{(2)}$ | $E^{(0)}$ | $E^{(2)}$ | |
| CN3 | 1 837 | −149.496 568 | −0.646 732(0) | −149.198 560 | −0.720 103(0) | 6.11 |
| | 3 654 | −149.662 402 | −0.386 269(0) | −149.368 197 | −0.420 330(2) | 7.08 |
| | 8 254 | −149.746 405 | −0.280 72(8) | −149.448 207 | −0.318 53(6) | 7.09 |
| | 19 311 | −149.810 865 | −0.207 1(2) | −149.516 943 | −0.237 31(9) | 7.18 |
| | 45 730 | −149.860 116 | −0.154 2(1) | −149.574 193 | −0.174 5(2) | 7.23 |
| | 108 321 | −149.897 832 | −0.115 52(8) | −149.616 166 | −0.131 2(1) | 7.24 |
| | 265 615 | −149.923 376 | −0.090 36(7) | −149.647 107 | −0.100 27(8) | 7.25 |
| | 713 756 | −149.942 653 | −0.071 80(7) | −149.669 387 | −0.078 73(7) | 7.25 |
| | 2 240 887 | −149.958 296 | −0.056 94(5) | −149.687 113 | −0.061 93(6) | 7.24 |
| | 8 287 086 | −149.972 592 | −0.043 27(4) | −149.702 834 | −0.047 39(5) | 7.23 |
| CN5 | 4 453 | −226.404 926 | −1.013 276(0) | −226.193 101 | −1.088 160(0) | 3.73 |
| | 8 818 | −226.591 687 | −0.685 258(5) | −226.372 170 | −0.743 445(6) | 4.39 |
| | 21 356 | −226.678 085 | −0.565 791(9) | −226.458 189 | −0.618 783(9) | 4.54 |
| | 51 557 | −226.751 503 | −0.473 218(8) | −226.533 681 | −0.519 42(1) | 4.67 |
| | 124 732 | −226.818 047 | −0.394 998(1) | −226.599 394 | −0.439 147(8) | 4.75 |
| | 306 926 | −226.879 535 | −0.326 711(1) | −226.662 318 | −0.366 750(1) | 4.82 |
| | 763 320 | −226.937 031 | −0.265 417(4) | −226.722 332 | −0.301 120(2) | 4.87 |
| | 1 912 184 | −226.988 127 | −0.212 58(1) | −226.778 410 | −0.242 12(2) | 4.90 |
| | 4 880 107 | −227.030 753 | −0.170 4(1) | −226.827 065 | −0.193 6(1) | 4.91 |
| | 13 631 497 | −227.063 119 | −0.140 20(8) | −226.866 875 | −0.155 6(1) | 4.92 |

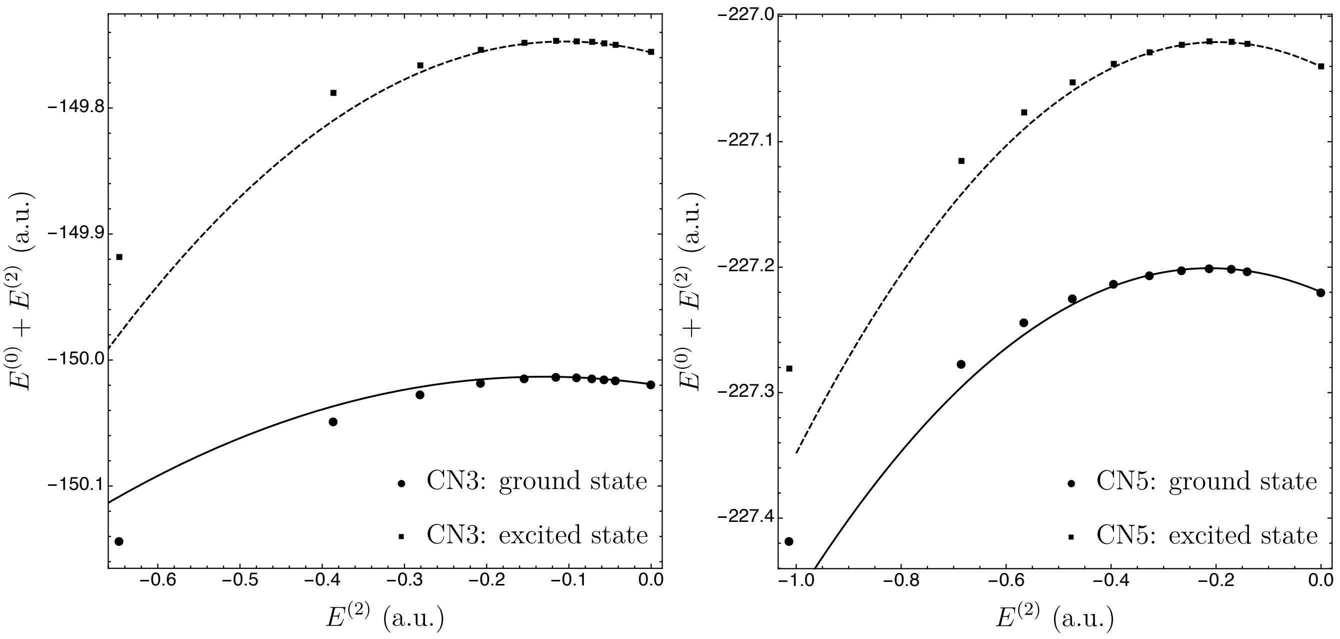


FIG. 2. Extrapolation of the sCI energies to the FCI limit (i.e. $E^{(2)} = 0$) for the ground state and the first singlet excited state of CN3 and CN5 obtained with the aug-cc-pVDZ basis set. The last five points (corresponding to the the five largest wave functions, that is, having the smallest $E^{(2)}$ values) are taken into account in the quadratic extrapolation.

**procedure** MS_SBK
  Perform CI calculation to get energies $E_k^{(0)}$ and coefficients $\boldsymbol{c}_k^{(0)}$ for $1 \leq k \leq N_{\text{st}}$
  Form $\boldsymbol{E}^{(0)} = \left(E_1^{(0)}, \ldots, E_{N_{\text{st}}}^{(0)}\right)$ and $\boldsymbol{c}^{(0)} = \left[\boldsymbol{c}_1^{(0)}, \ldots, \boldsymbol{c}_{N_{\text{st}}}^{(0)}\right]$
  $n \leftarrow 0$ ; $\boldsymbol{E}(n) \leftarrow \boldsymbol{E}^{(0)}$ ; $\Delta \boldsymbol{E} \leftarrow \infty$
  **while** $\max_k |\Delta E_k| > \tau$ **do** ▷ sBk iterations
    Build $\delta^{\text{sBk}}$ using Eq. (15b) ▷ $[N_{\text{det}} \times N_{\text{st}}]$
    $\boldsymbol{U} \leftarrow$ guess vectors ▷ $[N_{\text{det}} \times N_{\text{dav}}]$
    **for** $k = 1, \ldots, N_{\text{st}}$ **do**
      $\boldsymbol{U}_k \leftarrow \boldsymbol{c}^{(0)}$
    **end for**
    $\boldsymbol{R} \leftarrow \infty$
    **while** $\max_k \|R_k\| > \tau'$ **do** ▷ Davidson iterations
      Orthonormalize $\boldsymbol{U}$
      $\boldsymbol{W} \leftarrow \boldsymbol{H}.\boldsymbol{U}$ ▷ $[N_{\text{det}} \times N_{\text{dav}}]$
      $\boldsymbol{T} \leftarrow {}^{\dagger}\boldsymbol{c}^{(0)}.\boldsymbol{U}$ ▷ $[N_{\text{st}} \times N_{\text{dav}}]$
      $\boldsymbol{W} \leftarrow \boldsymbol{W} + \frac{1}{2}\,\delta^{\text{sBk}}.\boldsymbol{T}$
      $\boldsymbol{T}' \leftarrow {}^{\dagger}\delta^{\text{sBk}}.\boldsymbol{U}$ ▷ $[N_{\text{st}} \times N_{\text{dav}}]$
      $\boldsymbol{W} \leftarrow \boldsymbol{W} + \frac{1}{2}\,\boldsymbol{c}^{(0)}.\boldsymbol{T}'$
      $\boldsymbol{h} \leftarrow {}^{\dagger}\boldsymbol{U}.\boldsymbol{W}$ ▷ $[N_{\text{dav}} \times N_{\text{dav}}]$
      Diagonalize $\boldsymbol{h}$ to get energies $\boldsymbol{E}$ and eigenvectors $\boldsymbol{y}$
      Compute the residual $\boldsymbol{R}$ ▷ $[N_{\text{det}} \times N_{\text{st}}]$
      Append correction vectors to $\boldsymbol{U}$
      $N_{\text{dav}} \leftarrow N_{\text{dav}} + N_{\text{st}}$
    **end while**
    $\boldsymbol{y} \leftarrow$ the $N_{\text{st}}$ lowest eigenvectors in $\boldsymbol{y}$ ▷ $[N_{\text{det}} \times N_{\text{st}}]$
    $\boldsymbol{c}^{(0)} \leftarrow \boldsymbol{U}.\boldsymbol{y}$
    Compute $\boldsymbol{E}^{(0)}$ via Eq. (2) and set $\boldsymbol{E}(n) \leftarrow \boldsymbol{E}^{(0)}$
    Set $\Delta \boldsymbol{E} = \boldsymbol{E}(n) - \boldsymbol{E}(n-1)$ and $n \leftarrow n+1$
  **end while**
  **return** $\boldsymbol{E}$ and $\boldsymbol{c}^{(0)}$
**end procedure**

FIG. 3. Pseudo-code for the multi-state self-consistent shifted-Bk algorithm. The dimensions of the matrices are given as comments. $\tau$ and $\tau'$ are user-defined thresholds set as $10^{-5}$ and $10^{-10}$ respectively.
